# Supplementary material for: Inversion-Free Video Style Transfer with Trajectory Reset Attention Control and Content-Style Bridging
Source: arXiv:2503.07363 source file (2025-03-10)
Supplement: Supplementary file 1 [file X_suppl.tex]

\clearpage
\setcounter{page}{1}
\maketitlesupplementary

\section{High-Fidelity Visual Samples}
We provide additional visual comparisons between our method and other methods in \cref{fig: S1}, \cref{fig: S2}, \cref{fig: S3}, \cref{fig: S4}, \cref{fig: S5}, and \cref{fig: S6}. Additionally, a collection of first frames from video style transfer samples is presented in \cref{fig: variation} to showcase the performance of our method across various style images.

\begin{figure*}
\centering 
\includegraphics[width=0.98\textwidth]{pdf/supplementary/S1.pdf} 
\caption{Additional high-fidelity visual comparison of style transfer results with other methods.}
\label{fig: S1}
\end{figure*}

\begin{figure*}
\centering 
\includegraphics[width=0.98\textwidth]{pdf/supplementary/S2.pdf} 
\caption{Additional high-fidelity visual comparison of style transfer results with other methods.}
\label{fig: S2}
\end{figure*}

\begin{figure*}
\centering 
\includegraphics[width=0.98\textwidth]{pdf/supplementary/S3.pdf} 
\caption{Additional high-fidelity visual comparison of style transfer results with other methods.}
\label{fig: S3}
\end{figure*}

\begin{figure*}
\centering 
\includegraphics[width=0.98\textwidth]{pdf/supplementary/S4.pdf} 
\caption{Additional high-fidelity visual comparison of style transfer results with other methods.}
\label{fig: S4}
\end{figure*}

\begin{figure*}
\centering 
\includegraphics[width=0.98\textwidth]{pdf/supplementary/S5.pdf} 
\caption{Additional high-fidelity visual comparison of style transfer results with other methods.}
\label{fig: S5}
\end{figure*}

\begin{figure*}
\centering 
\includegraphics[width=0.98\textwidth]{pdf/supplementary/S6.pdf} 
\caption{Additional high-fidelity visual comparison of style transfer results with other methods.}
\label{fig: S6}
\end{figure*}

\begin{figure*}
\centering 
\includegraphics[width=\textwidth]{pdf/supplementary/variations.png} 
\caption{Additional video style transfer samples under various style images.}
\label{fig: variation}
\end{figure*}

\section{Source Attributions}

We provide links to the assets used in this paper. Unless explicitly mentioned otherwise, all other sources were collected from \href{https://pixabay.com/}{Pixabay}.

\begin{table}[ht]
    \centering
    
    \small

    \label{tab: asset_source}
    \begin{tabular}{c | l}
        \toprule
        \cref{fig: style medium} & 
        (row 1) \href{https://pixabay.com/zh/videos/woman-sea-rocks-beach-island-148597/}{1}; 
        (row 2) \href{https://pixabay.com/zh/videos/pear-tree-blossom-bloom-35735/}{1},\href{https://www.shetu66.com/muban/566581811858247913}{2};
        (row 3) \href{https://pixabay.com/zh/videos/drone-flying-object-flying-119278/}{1},\href{https://www.behance.net/gallery/120147773/Le-Chum-Bucket}{2}; 
        (row 4) \href{https://pixabay.com/zh/videos/parrot-bird-animal-plumage-23223/}{1},\href{https://www.68design.net/work/716729}{2};\\
        
        \cref{fig: comparison} & 
        (row 1) \href{https://pixabay.com/zh/videos/drone-flying-object-flying-119278/}{1},\href{https://www.zcool.com.cn/work/ZNDI2NDUyMjg=.html}{2},\href{https://pixabay.com/zh/videos/pear-tree-blossom-bloom-35735/}{8},\href{https://www.researchgate.net/publication/380616806_A_Comparative_Study_on_the_Painting_Forms_of_Western_Oil_Painting_and_Chinese_Ink_Painting}{9}; 
        (row 5) \href{https://pixabay.com/zh/videos/robot-android-3d-cartoon-surf-141984/}{1},\href{https://www.zcool.com.cn/work/ZMzY0OTQ5NzI=.html}{2},\href{https://pixabay.com/zh/videos/ship-vessel-sea-boat-ocean-water-237249/}{8},\href{https://www.zcool.com.cn/work/ZMjM1NTUxNjA=.html}{9}; 
        % (row 3) \href{}{1},\href{}{2},\href{}{8},\href{}{9}; 
        % (row 4) \href{}{1},\href{}{2},\href{}{8},\href{}{9};
        \\
        
        \cref{fig: restrict} & (right side, row 2) \href{https://www.zcool.com.cn/work/ZMTc0ODU1ODQ=.html}{1};\\
        
        \bottomrule
    \end{tabular}
    \caption{Asset sources.}
\end{table}

\section{Justification of Experiment Settings}
All results from the comparison methods were obtained by running the official code provided, using the recommended settings. In contrast, our method offers a variety of tunable parameters at inference, allowing for adjustments such as controlling the degree of style, managing content preservation, and enhancing the consistency of details. These tunable settings enable our approach to achieve better performance on specific samples, and we recommend utilizing them for optimal results. However, for a fair comparison, all results from our proposed method were generated using a consistent set of parameters.

The collected benchmark dataset comprises 20 videos and 20 style images spanning various categories. For the experiments, a total of 400 videos were generated to assess performance. 
The efficiency comparison experiment measured the average processing speed using a 20-frame video at a resolution of $512\times512$, executed on an NVIDIA RTX A6000 GPU.

% \section{Rationale}
% \label{sec:rationale}
% % 
% Having the supplementary compiled together with the main paper means that:
% % 
% \begin{itemize}
% \item The supplementary can back-reference sections of the main paper, for example, we can refer to \cref{sec:intro};
% \item The main paper can forward reference sub-sections within the supplementary explicitly (e.g. referring to a particular experiment); 
% \item When submitted to arXiv, the supplementary will already included at the end of the paper.
% \end{itemize}
% % 
% To split the supplementary pages from the main paper, you can use \href{https://support.apple.com/en-ca/guide/preview/prvw11793/mac#:~:text=Delete%20a%20page%20from%20a,or%20choose%20Edit%20%3E%20Delete).}{Preview (on macOS)}, \href{https://www.adobe.com/acrobat/how-to/delete-pages-from-pdf.html#:~:text=Choose%20%E2%80%9CTools%E2%80%9D%20%3E%20%E2%80%9COrganize,or%20pages%20from%20the%20file.}{Adobe Acrobat} (on all OSs), as well as \href{https://superuser.com/questions/517986/is-it-possible-to-delete-some-pages-of-a-pdf-document}{command line tools}.
